# Supplementary material for: LLMs Can't Plan, But Can Help Planning in LLM-Modulo Frameworks
Source: arXiv:2402.01817 source file (2024-06-12)
Supplement: Supplementary file 1 [file Appendix.tex]

\newpage
\appendix
\onecolumn
\section{You \emph{can} have an appendix here.}

You can have as much text here as you want. The main body must be at most $8$ pages long.
For the final version, one more page can be added.
If you want, you can use an appendix like this one.  

The $\mathtt{\backslash onecolumn}$ command above can be kept in place if you prefer a one-column appendix, or can be removed if you prefer a two-column appendix.  Apart from this possible change, the style (font size, spacing, margins, page numbering, etc.) should be kept the same as the main body.
